# Supplementary material for: Microscopic origin of the effective spin-spin interaction in a semiconductor quantum dot ensemble
Source: arXiv:2207.02707 source file (2022-07-19)
Supplement: Supplementary file 1 [file supplement.pdf]

# Supplement to "Microscopic origin of the effective spin-spin interaction in a semiconductor quantum dot ensemble"

Frederik Vonhoff,[1] Andreas Fischer,[1] Kira Deltenre,[1] and Frithjof B. Anders[1]

[1] *Department of Physics, TU Dortmund University, Otto-Hahn-Straße 4, 44227 Dortmund, Germany*

(Dated: July 5, 2022)

In this supplement, we provide a summary of the applied methods in particular some details of the numerical renormalization group (NRG) approach that might be important when reproducing our findings. The details of the conventional implementation concerning the applied methods can be found in the literature.

## I. WILSON CHAIN CONSTRUCTION FOR AN ASYMMETRIC WETTING LAYER BAND

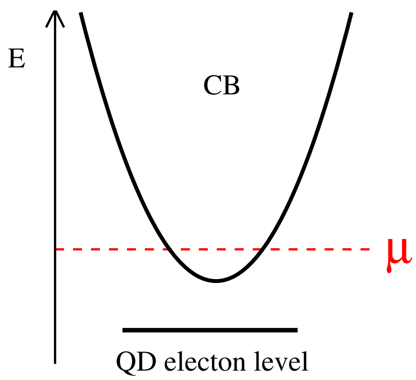


FIG. S1. Cartoon of the quantum dot (QD) level, the quadratic wetting layer (WL) band dispersion, and the chemical potential $\mu$ located very close the bottom of the wetting layer.

The energy hierarchy of our setup is plotted in Fig. S1. The quantum dot (QD) orbital energy lies below the lower band edge of the wetting layer (WL), and the chemical potential is very low due to very low band filling. The band cutoff energy scale in the NRG has been set to $D = 1$eV while the $\Gamma$-point is located at $E = 0$ and $1meV > \mu > 0$. A finite Coulomb repulsion $U$ prevents the QD level to be doubly occupied when the energy of the doubly occupied state exceeds the energy of the singly occupied QD level: $\varepsilon^d + U > \mu$.

Klein and Fischer [1] calculated the effective RKKY interaction between two localized spin 1/2 with a distance $R = |\vec{R}|$ apart coupled by a Kondo Hamiltonian to a 2D conduction band with a quadratic dispersion at low band filling. They perturbatively derived the formula,

$$J_{ij}^{\mathrm{RKKY}} = -\rho_0 \bar{J}_K^2 \frac{\bar{v} k_F^2}{4\pi} \times \left[ J_0(k_F R) N_0(k_F R) + J_1(k_F R) N_1(k_F R) \right], \tag{S1}$$

which is stated in our letter. The Bessel (Neumann) function $J_l(x)(N_l(x))$ of order $l$ enters as well as the area $\bar{v}$ of the 2D unit cell. The prefactor $\rho_0 \bar{J}_K^2 \frac{\bar{v} k_F^2}{4\pi}$ determines the overall strength.

Our model, however, starts from a single particle hybridization term that also includes charge fluctuation. It is known in the literature [2, 3] that a two stage approximation, i. e. first performing a Schrieffer-Wolff transformation to obtain an effective local Kondo interaction and then using Eqn. (S1) in the second step is inconsistent in some parameter regime, such as short distance and small hybridization $V_0$, since not all terms in order $O(V_0^4)$ are accounted for. The additional contribution neglected in this two stage approach, however, can have a significant impact on the results. Therefore, we employed Wilson's numerical renormalization group (NRG) approach [4, 5] in order to obtain a non-perturbative RKKY interaction function $J_{12}^{\mathrm{RKKY}}(R)$ between the localized electron spins of two QD.

The scenario plotted in Fig. S1 is very unusual and typically not addressed by standard NRG calculations. It is characterized by a very asymmetric density of states of the WL band whose support is defined by the interval $I_A = [-\mu : D]$. Since $\mu/D \ll 1$, it is very challenging to construct the appropriate Wilson chain. The reason is that the scaling of the tight-binding hopping parameter change their scaling from $t_n \propto \Lambda^{-n/2}$ for $\mu/D = O(1)$ to $t_n \propto \Lambda^{-n}$ for $\mu \leq 0$ which is the same scaling as for the bosonic NRG [6, 7]. This change of scaling is caused by the absence of hole excitations for $\mu < 0$ or the requirement of $\omega > 0$ in the harmonic oscillator. The discretiation of the NRG is parametrized by $\Lambda > 1$, and $n$ denotes the chain site.

The question arises what happens in the limit $\mu \to 0^+$. To the best of our knowledge, that question was addressed in a diploma thesis by Hager [8] supervised by Ralf Bulla for the first time. In his thesis, Hager proposed an alternative discretization scheme adapted to the strongly asymmetric support of the conduction band continuum. We, however, used the Wilson's standard discretization summarized in the NRG review [5] which used a symmetric support $I_S = [-D : D]$ but supplying an energy dependent density of states which is only finite on $I_A$ and zero otherwise. It turns out that our Wilson chain parameters are more or less identical with those derived by Hager indicating that the mapped model contains the same physics.

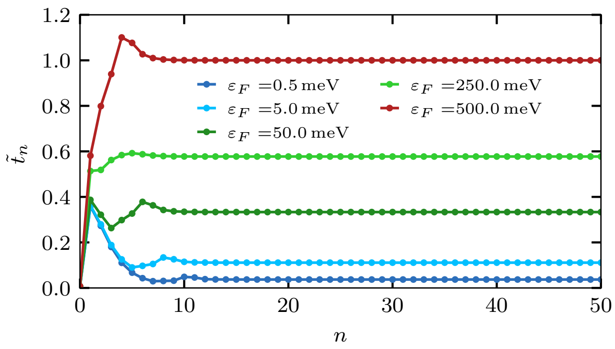


FIG. S2. Scaled hopping elements $\tilde{t}_n$ of the Wilson chain vs iteration number $n$ for different Fermi energies $\varepsilon_F$.

We plotted the dimensionsless Wilson chain hopping parameters using in our NRG calculations for a two-impurity Anderson model [2, 3] in Fig. S2 where $\tilde{t}_n = t_n 2\Lambda^{(n-1)/2}/(D(1+\Lambda^{-1}))$ vs the NRG interaction index $n$ for various values of $\mu$ are shown for $\Lambda = 3$ and $D = 1\,\text{eV}$. Clearly visible are the fixed points for large $n$. The hopping parameters at the fixed points do not depend on the distance $R$ and are only governed by the ratio $\mu/D$. For $\mu = O(D)$, $\tilde{t}_n \to 1$ for large $n$ as established by Wilson [9]. When decreasing $\mu \leq 0.25\,\text{eV}$, $\tilde{t}_n$ is reduced as already reported by Hager [8]. Since the NRG fixed point spectrum is proportional to $\tilde{t}_\infty$ [4] ($\tilde{t}_\infty = \lim_{n\to\infty} \tilde{t}_n$), the NRG eigenenergies $\bar{E}_j$ are strongly reduced for small chemical potentials.

The thermodynamic expectation values of the operator $\hat{O}$ are calculated by

$$\langle \hat{O} \rangle (T_n) = \frac{1}{Z_n} \sum_j e^{-\beta_n E_j} \langle j | \hat{O} | j \rangle \qquad \text{(S2)}$$

$$Z_n = \sum_j e^{-\beta_n E_j} \qquad \text{(S3)}$$

where $T_n \propto \Lambda^{-(n-1)/2}$, and $j$ denotes all eigenstates of $H$ present at the iteration $n$. By reducing the temperature $T_n$ in each iteration step [5], $\beta_n E_j = \bar{\beta} \bar{E}_j$ is used in the NRG approach. Operating with rescale energies $\bar{E}_j \propto \Lambda^{n/2} E_j$ at each NRG interation, one uses a fixed $\bar{\beta} = O(1)$ [9]. Since $\bar{E}_j \propto \tilde{t}_\infty$ at the fixed point, we need to adjust $\bar{\beta} \approx 1/\tilde{t}_\infty$ in order to reliably evaluate Eq. (S2) using only the NRG states present at iteration $n$. It turns out that $\tilde{t}_\infty$ only depends on $\mu$ and not on $R$ since the asymptotic value is determined by the support of $\rho(\omega)$ only. Therefore, we can fix $\bar{\beta}$ for a given $\mu$ independent of the distance $R$. In the letter, we used $\bar{\beta} = 40$ for all NRG calculations after checking that slight variations of $\bar{\beta}$ do not change the results.

## II. FITTING THE NRG DATA TO THE TOY MODEL

The two impurity Anderson model has a few unstable fixed points (FP). It contains the free orbital FP at high temperatures which flows towards the local moment (LM) FP for the parameter regime relevant in this paper: We consider QD binding energy $\varepsilon^d$ and Coulomb repulsion $U$ such that the QDs are singly occupied at low temperatures.

Once the LM regime is established, and the Kondo temperature is well below the $J^{\text{RKKY}}$, either a correlated local triplet or a singlet is formed by the two impurity spins. In case of a triplet, the system undergoes a two stage Kondo effect to eventually form a Kondo singlet out of the $S = 1$ local triplet. If an RKKY singlet is formed, it decouples from the remaining low energy degrees of freedom of the conduction band and the Kondo effect is absent. The two types of FPs can be separated by the NRG energy spectrum [10]. Note however, there is no quantum phase transition between these two fixed points as pointed out by Affleck et al. [11]. The Jones-Varma quantum critical point (QCP) [10] is an artifact to their approximation [10] while the particle-hole asymmetry generates a relevant perturbation in the correct treatment [11]: only a continuous crossover between these FPs is observed. The low temperature FP is always a singlet in more than one dimension [3, 12] since it belongs to a the multi-impurity Anderson model class of first kind – see Eickhoff and Anders [12] for more details.

In this paper, we usually select parameters such that the two-stage Kondo effect occurs below the relevant energy scale of the effective RKKY scale. We aim for the extraction of $J^{\text{RKKY}}(R)$ from the NRG impurity entropy as well as the temperature dependent spin-spin correlation function $\langle \vec{S}_1 \vec{S}_2 \rangle$ between the electron spins localized in the two QDs. The crossover between the different unstable FPs is illustrated for three different distances $R$ with effective ferromagnetic (FM) $J^{\text{RKKY}}$ in Fig. S3(a) that depicts the temperature dependency of the impurity entropy [4, 5]. Starting at the free orbital FP $\log(g) = \log(16)$, the degeneracy is lifted after cooling below $U$, and two LMs, one in each QD is formed, are leading to $S_{\text{imp}} = \log(4)$. We observe a crossover to $S_{\text{imp}} = \log(3)$ indicating the triplet formation due to $J^{\text{RKKY}} < 0$. Reducing the temperature further leads to $S_{\text{imp}} = \log(2)$ after the Kondo screening of one of the two effective conduction bands sets in. The larger the difference in the conduction band coupling the later the second screening sets in, and the ground state singlet is formed, i. e. $S_{\text{imp}} = \log(1) = 0$.

For extracting the $J^{\text{RKKY}}$, we focus on the crossover from the LM formation until $\langle \vec{S}_1 \vec{S}_2 \rangle$ reached its low temperature fixed point value, while still being well above the Kondo scale. Let us assume for a moment that the dominating residual interaction is a dynamically generated $J^{\text{RKKY}}$ around the LM FP. Then the FP Hamiltonian could be approximated by a two-spin model with an in-

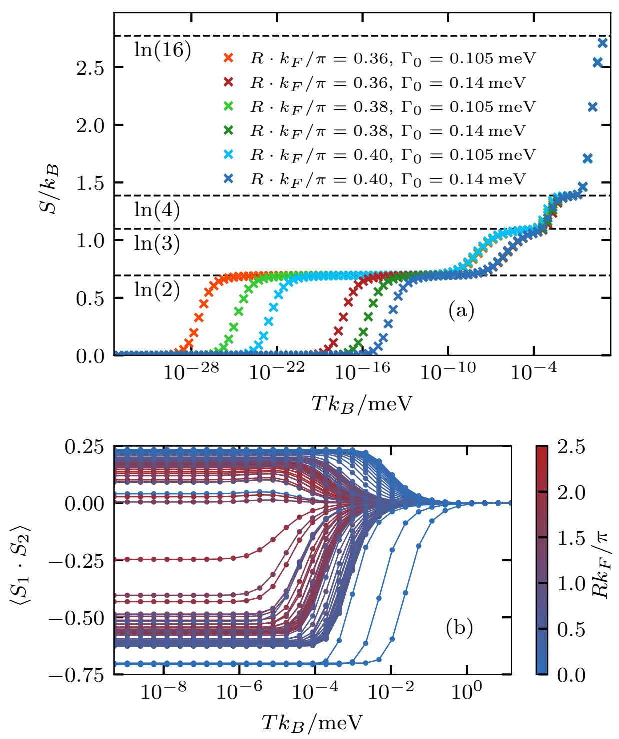


FIG. S3. (a) Entropy $S/k_B$ vs temperature $Tk_B$ for different distances $Rk_F/\pi$ and $\Gamma_0$. The dashed black lines indicate relevant logarithmic values for the steplike increase of the entropy. (b) Correlation function $C_{12}(T,R) = \langle \vec{S}_1 \vec{S}_2 \rangle (T,R)$ vs temperature $Tk_B$ for different distances $Rk_F/\pi$. NRG parameter: $\Lambda = 5$, $D = 1\,\text{eV}$, $\bar{\beta} = 40$, $N_{\text{kp}} = 3000$ (number of kept eigenstates,) and $N = 100$ (number of iterations) for (a) and $N = 32$ for (b).

teraction $H_{\text{eff}} = J\vec{S}_1\vec{S}_2$ and two decoupled conduction bands. The eigenstates are a singlet and a triplet, and the local spin correlation function is given by

$$S_{12}(T) = \langle \vec{S}_1 \vec{S}_2 \rangle = -\frac{3}{4}\left(\frac{1-e^{-\beta J}}{1+3e^{-\beta J}}\right) = -s(s+1)\left(\frac{1-e^{-\beta J}}{1+3e^{-\beta J}}\right) \tag{S4}$$

for two interacting $s = 1/2$ spins. We clearly see that for $J > 0$, $\lim_{T\to 0} S_{12}(T) = -3/4$ and for $J < 0$, $\lim_{T\to 0} S_{12}(T) = 1/4$.

When the local Kondo coupling would be very small, we could fit our NRG data to Eq. (S4) and identified the fit parameter $J$ with $J^{\text{RKKY}}(R)$ for each $R$. This is not always the case. We operate in a regime where $\Gamma_0$ and $J^{\text{RKKY}}(R)$ are relatively small numbers compared to $U$ that is responsible for forming the LM FP. The Schrieffer-Wolff transformation[13], however, yields a $J_K \approx 4V_0^2/U$ that is of the order of 1 eV. Clearly, one cannot take this value seriously since the notion of a Kondo coupling only makes sense if $|J_K| < U$, i. e. on an energy scale after the LM has been formed. That requires $T_n < U$. Consequently, we did not discuss the value of $J_K$ in the letter since the concept of a LM coupling constant $J_K \approx D$ is somehow meaningless when the LMs are only generated below $U = 4\,\text{meV}$.

This observation, however, indicates that around the LM FP, where $S_{\text{imp}} = \log(4)$, there are two types of perturbations of the FP present: $J^{\text{RKKY}}(R)$ which is trying to lock the electron spins of two QDs to a singlet or a triplet, and an effective $J_K$ at each QD location tries to screen the LM. For a substantial $J_K$, we expect that the screening of the LMs sets in well above the Kondo temperature of the problem and even affects the singlet formation.

While the LM FP is clearly characterized by two spin 1/2 degrees of freedom, the renormalization group calculation changes the operator content of the local spins. By the onset of the local screening process, the localized electrons contribute less and bound conduction electron spins are contributing instead. Since we track the local spin-spin correlation functions $S_{12}(T)$, the reduction of the spin matrix elements reduced the maximal amplitude of $S_{12}(T)$.

To illustrate the effect of the dynamically generated $J^{\text{RKKY}}(R)$ in the presence of a Kondo coupling, we plotted temperature dependent spin-spin correlation functions $S_{12}(T)$ for a series of different distances $Rk_F/\pi = 0.02 \cdot n < 2.5$ with $n \in \mathbb{N}_0$ in Fig. S3(b). While for short distances, $S_{12}(T \to 0)$ almost approaches one of the two theoretical asymptotic values $1/4$ or $-3/4$, these values decrease with increasing distance $R$. This observation in the NRG calculated correlation function can be understood very easily: while the local $J_K$ is distance independent, $J^{\text{RKKY}}(R) \propto 1/R^2$. With increasing distance, the $J^{\text{RKKY}}(R)$ induced spin-spin correlation occurs at decreasing temperature as can be seen in Fig. S3(b). Therefore, the local Kondo screening already sets in, and the renormalization group calculation yields a reduction of the effective moment $\mu_{\text{eff}}^2(T)$. At temperatures around $T \approx U$, $\mu_{\text{eff}}^2 = s(s+1)$, but when $T \approx J^{\text{RKKY}}(R)$, $\mu_{\text{eff}}^2$ is renormalized and potentially reduced. Therefore, we used the two parameter fit function

$$S_2(T) = -\mu_{\text{eff}}^2 \left(\frac{1-e^{-\beta J}}{1+3e^{-\beta J}}\right) \tag{S5}$$

to extract $J^{\text{RKKY}}(R)$ from the NRG data absorbing the reduced LM into the second fit parameter $\mu_{\text{eff}}^2$.

Assuming that we can replace $\mu_{\text{eff}}^2(T)$ by a constant value when $T \approx J^{\text{RKKY}}(R)$, we can (i) extract $\mu_{\text{eff}}^2(J^{\text{RKKY}}(R))$ by fitting $S_2(T)$ to the $T \to 0$ asymptotic values, and then (ii) replace $s(s+1) \to \mu_{\text{eff}}^2(J^{\text{RKKY}}(R))$ in Eq. (S4) for extracting $J^{\text{RKKY}}(R)$ by fitting the temperature dependence to the modified Eq. (S4).

The NRG parameters are set to $\Lambda = 5$, $D = 1\,\text{eV}$, $\bar{\beta} = 40$, $N_{\text{kp}} = 3000$ (number of kept eigenstates), and $N = 100$ (number of iterations) for (a) and $N = 32$ for (b). The model parameter are chosen to be $\Gamma_0 = 0.14\,\text{meV}$,

$\varepsilon_F = 0.5\,\text{meV}$, $U = 4\,\text{meV}$ and $\varepsilon_d = -1.5\,\text{meV}$. The RKKY interaction for the chosen distances in figure S3 (a) is always FM so that the unstable ln(3) level can be observed. The correlation functions in Fig. S3 (b) are printed for different distances $Rk_F/\pi = 0.02 \cdot n < 2.5$ with $n \in \mathbb{N}_0$.

## III. SIMULATION OF THE SPIN DYNAMICS IN LASER PULSED QD ENSEMBLES

In the simulation of the spin dynamics in the QD ensemble governed by the central spin model $H_1^{(i)}$,

$$H_1^{(i)} = g_e^{(i)} \mu_{\text{B}} \vec{B}_{\text{ext}} \vec{S}^{(i)} + \sum_k g_{N,k}^{(i)} \mu_{\text{N}} \vec{B}_{\text{ext}} \vec{I}_k^{(i)} + \sum_{k=1}^{N_i} A_k^{(i)} \vec{I}_k^{(i)} \vec{S}^{(i)}, \tag{S6}$$

for each QD augmented with an inter QD Heisenberg coupling,

$$H_{\text{array}} = \sum_i^{N_{QD}} H_1^{(i)} + \sum_{i<j} J_{ij} \vec{S}^{(i)} \vec{S}^{(j)}, \tag{S7}$$

we replace all quantum mechanical spins by a classical vector. Furthermore, we also take into account a trion state excited by the laser pulse and treat the spin/trion system with a Lindblad approach to accommodate the radiative decay of the trion into the spin state, which results in the equations of motion

$$\partial_t \vec{s}^{(i)} = \left( g_e^{(i)} \mu_{\text{B}} \vec{B}_{\text{ext}} + \sum_{k=1}^{N_i} A_k^{(i)} \vec{i}_k^{(i)} + \sum_{j=1}^{N_{QD}} J_{ij} \vec{s}^{(j)} \right) \times \vec{s}^{(i)} \tag{S8}$$

$$+ \frac{1}{2} \gamma p_T^{(i)} \vec{e}_z \tag{S9}$$

$$\partial_t \vec{i}^{(i)} = \left( g_{N,k}^{(i)} \mu_{\text{N}} \vec{B}_{\text{ext}} + A_k^{(i)} \vec{s}^{(i)} \right) \times \vec{i}_k^{(i)} \tag{S10}$$

$$\partial p_T^{(i)} = -\gamma p_T^{(i)} \, . \tag{S11}$$

Here $\vec{s}^{(i)}, \vec{i}^{(i)} \in \mathbb{R}^3$ are the classical vectors corresponding to the operators $\vec{S}^{(i)}, \vec{I}_k^{(i)}$ while $p_T^{(i)}$ is the trion occupation probability, and $\gamma = 10\text{ns}^{-1}$ denotes the trion decay rate. For the initial conditions, $\vec{s}^{(i)}$ and $\vec{i}^{(i)}$ are drawn uniformly from the Bloch-sphere while the trion occupation is set to zero. This meets the situation that at cryostatic temperatures, where $k_B T$ is larger than any energy scale in Hamiltonian (S7), but $k_B T$ is significantly smaller than the trion excitation energy. The effect of an instantaneous resonant $\pi$ pulse with $\sigma^+$ polarization at time $t$ on QD $i$ can be summerized by

$$\vec{s}^{(i)}(t^+) = \frac{1}{2} \left( \vec{s}_z^{(i)}(t^-) - \frac{1}{2} \right) \vec{e}_z \tag{S12}$$

$$p_T^{(i)}(t^+) = \vec{s}_z^{(i)}(t^-) + \frac{1}{2} \, , \tag{S13}$$

where $t^+$ is the time right after the pulse and $t^-$ is the time right before the pulse. The background of the approximations, the justification, the technical details and treatment of the laser pulse are very elaborately explained in Ref. [14] and applied to a QD ensemble in Ref. [15]. The semiclassical equations of motion can also be derived in a saddle point approximation from a path integral formulation [16] which allows to properly include nuclear-electric quadrupolar interactions [17] in the semiclassical dynamics. We did not include the quadrupolar interactions since they are only relevant on timescale larger than 100ns.

We use the linearly increasing phase shift reported in Ref. [18] as a benchmark for the distance dependent interaction strength $J^{\text{RKKY}}(R)$. The phase shift not only provides an estimate for the magnitude of the interaction, but is also sensitive to the distribution of the coupling constants. This becomes clear when studying at the analytic solution for the phase shift of two QDs with fixed interaction strength $J$. It results in the temporal phase shift

$$\phi(t) = \arccos\left( \frac{1 + \cos(\frac{J}{\sqrt{2}} t)}{\sqrt{2 + 2\cos^2(\frac{J}{\sqrt{2}} t)}} \right) = \frac{J^2 t^2}{8} + O((Jt)^4) \tag{S14}$$

which increases quadratically for short times and thus deviates from the experimental result. However, by averaging different coupling strengths the nearly linear regime can be restored. Since not only the interaction strength but also the distribution of the coupling constants is relevant for the reproduction of the experimental results, a match is particularly promising.


[1] B. Fischer and M. W. Klein, Magnetic and nonmagnetic impurities in two-dimensional metals, Phys. Rev. B **11**, 2025 (1975).

[2] R. Žitko and J. Bonča, Multiple-impurity anderson model for quantum dots coupled in parallel, Phys. Rev. B. **74**, 045312 (2006).

[3] F. Eickhoff, B. Lechtenberg, and F. B. Anders, Effective low-energy description of the two-impurity Anderson model: RKKY interaction and quantum criticality, Phys. Rev. B **98**, 115103 (2018).

[4] H. R. Krishna-murthy, J. W. Wilkins, and K. G. Wilson, Renormalization-group approach to the Anderson model of dilute magnetic alloys. I. Static properties for the symmetric case, Phys. Rev. B **21**, 1003 (1980).

[5] R. Bulla, T. A. Costi, and T. Pruschke, The numerical renormalization group method for quantum impurity systems, Rev. Mod. Phys. **80**, 395 (2008).

[6] R. Bulla, N.-H. Tong, and M. Vojta, Numerical renormalization group for bosonic systems and application to the sub-ohmic spin-boson model, Phys. Rev. Lett. **91**, 170601 (2003).

[7] R. Bulla, H.-J. Lee, N.-H. Tong, and M. Vojta, Numerical renormalization group for quantum impurities in a bosonic bath, Phys. Rev. B **71**, 045122 (2005).

[8] R. Hager, *Kondo-Effekt in Systemen mit niedriger Ladungsträgerkonzentration*, Master's thesis, Department of Physics, University of Augsburg (2007).

[9] K. G. Wilson, Rev. Mod. Phys. **47**, 773 (1975).

[10] B. A. Jones and C. M. Varma, Study of two magnetic impurities in a Fermi gas, Phys. Rev. Lett. **58**, 843 (1987).

[11] I. Affleck, A. W. W. Ludwig, and B. A. Jones, Conformal-field-theory approach to the two-impurity Kondo problem: Comparison with numerical renormalization-group results, Phys. Rev. B **52**, 9528 (1995).

[12] F. Eickhoff and F. B. Anders, Strongly correlated multi-impurity models: The crossover from a single-impurity problem to lattice models, Phys. Rev. B **102**, 205132 (2020).

[13] J. R. Schrieffer and P. A. Wolff, Relation between the Anderson and Kondo Hamiltonians, Phys. Rev. **149**, 491 (1966).

[14] N. Jäschke, A. Fischer, E. Evers, V. V. Belykh, A. Greilich, M. Bayer, and F. B. Anders, Nonequilibrium nuclear spin distribution function in quantum dots subject to periodic pulses, Phys. Rev. B **96**, 205419 (2017).

[15] A. Fischer, E. Evers, S. Varwig, A. Greilich, M. Bayer, and F. B. Anders, Signatures of long-range spin-spin interactions in an (In,Ga)As quantum dot ensemble, Phys. Rev. B **98**, 205308 (2018).

[16] G. Chen, D. L. Bergman, and L. Balents, Semiclassical dynamics and long-time asymptotics of the central-spin problem in a quantum dot, Phys. Rev. B **76**, 045312 (2007).

[17] A. Fischer, I. Kleinjohann, N. A. Sinitsyn, and F. B. Anders, Cross-correlation spectra in interacting quantum dot systems, Phys. Rev. B **105**, 035303 (2022).

[18] S. Spatzek, A. Greilich, S. E. Economou, S. Varwig, A. Schwan, D. R. Yakovlev, D. Reuter, A. D. Wieck, T. L. Reinecke, and M. Bayer, Optical Control of Coherent Interactions between Electron Spins in InGaAs Quantum Dots, Phys. Rev. Lett. **107**, 137402 (2011).
